# Supplementary material for: Code Documentation and Analysis to Secure Software Development
Source: arXiv:2407.11934 source file (2024-07-16)
Supplement: Supplementary file 1 [file appendices.tex]

\clearpage

\appendix

%Appendices
% 1. Userguide for CoDAT 
% 2. Link to Example Code
% 3. Link to Project Code
% 4. AI program output 

%\section{User manual for CoDAT}
\input{manual}

\section{Example Project Code}

% Project code used as an example 

\section{Appendix Plugin Code}

% Source code for plugin here along with link for full implementation (Boilerplate, etc.)
